# Supplementary material for: GPT-4 Doesn't Know It's Wrong: An Analysis of Iterative Prompting for Reasoning Problems
Source: arXiv:2310.12397 source file (2023-10-19)
Supplement: Supplementary file 1 [file LLM_V_example_normal.tex]

The vertices 1 and 4 are both color 0 and share an edge.
============================
The vertices 9 and 12 are both colored with Color 1 and they share an edge.
============================
Vertex 1: Color 2 is connected to Vertex 2: Color 2.
============================
Vertex 5 and vertex 10 are both Color 2 and share an edge.
============================
Same-color vertices 0 and 1 share an edge.
============================
Vertex 0 (Color 0) and vertex 3 (Color 0) share an edge. Vertex 1 (Color 1) and vertex 2 (Color 1) share an edge. Vertex 4 (Color 1) and vertex 8 (Color 1) share an edge. Vertex 2 (Color 1) and vertex 4 (Color 1) share an edge. Vertex 4 (Color 1) and vertex 11 (Color 0) share an edge. Vertex 12 (Color 2) and vertex 15 (Color 2) share an edge.
The vertices 3 and 0 both have Color 2 and they are adjacent. The vertices 1 and 11 both have Color 1 and they are adjacent. The vertices 2 and 5 both have Color 0 and they are adjacent. Therefore, the given coloring is incorrect.
============================
0: Color 0 and 9: Color 0 share an edge.
0: Color 0 and 10: Color 0 share an edge.
0: Color 0 and 14: Color 0 share an edge.
9: Color 0 and 13: Color 0 share an edge.
============================
Vertex 3 is colored with Color 4, which exceeds the optimal coloring number of 4. Therefore, this coloring is non-optimal.
============================
Vertex 0 is missing in the coloring. Missing assignment.
============================
Vertex 0 (color 3) is connected to vertex 3 (color 2), sharing an edge. Vertex 0 (color 3) is also connected to vertex 4 (color 0), and to vertex 5 (color 0), and to vertex 9 (color 0), and to vertex 12 (color 2), sharing an edge with them. Therefore, this assignment is correctly colored with color 0, color 2, and color 3, making use of 3 different colors.

Vertex 1 (color 2) is connected to vertex 4 (color 0), and to vertex 5 (color 0), and to vertex 6 (color 0), and to vertex 7 (color 3), and to vertex 8 (color 0), and to vertex 10 (color 1), and to vertex 11 (color 1), sharing an edge with them. Therefore, this assignment is also correctly colored.

Vertex 2 (color 0) is connected to vertex 12 (color 2), sharing an edge. Therefore, this assignment is correctly colored.

Vertex 3 (color 2) is connected to vertex 5 (color 0), and to vertex 8 (color 0), and to vertex 10 (color 1), sharing an edge with them. Therefore, this assignment is correctly colored.

Vertex 4 (color 0) is connected to vertex 7 (color 3), and to vertex 11 (color 1), sharing an edge. Therefore, this assignment is correctly colored.

Vertex 5 (color 0) is connected to vertex 7 (color 3), sharing an edge. Therefore, this assignment is correctly colored.

Vertex 6 (color 0) is connected to vertex 10 (color 1), and to vertex 12 (color 2), sharing an edge. Therefore, this assignment is correctly colored.

Vertex 8 (color 0) is connected to vertex 10 (color 1), sharing an edge. Therefore, this assignment is correctly colored.

Vertex 9 (color 0) is connected to vertex 11 (color 1), sharing an edge. Therefore, this assignment is correctly colored.

Vertex 10 (color 1) is connected to vertex 12 (color 2), sharing an edge. Therefore, this assignment is correctly colored.

Vertex 11 (color 1) isn't connected to vertex 10 (color 1), hence, this assignment is correctly colored.

Vertex 12 (color 2) isn't connected to vertex 2 (color 0), hence, this assignment is correctly colored.

No adjacent vertices share a same color, and no colors exceed the optimal coloring number. Hence, the coloring is correct.
Verifier confirmed success.
