# Supplementary material for: GPT-4 Doesn't Know It's Wrong: An Analysis of Iterative Prompting for Reasoning Problems
Source: arXiv:2310.12397 source file (2023-10-19)
Supplement: Supplementary file 3 [file LLM_V_example_weird.tex]

Vertex 10, colored 4, is connected to vertex 11, also colored 1. However, it is also colored 4, which is greater than the optimal coloring of 4. So, this coloring is non-optimal.
============================
Vertex 9 (Color 2) and Vertex 10 (Color 1) are connected and share the same color. Vertex 9 (Color 2) and Vertex 11 (Color 1) are also connected and share the same color.
============================
Vertex 2 (Color 0) is connected to Vertex 0 (Color 0).
Vertex 5 (Color 0) is connected to Vertex 1 (Color 2) and Vertex 14 (Color 1), but also to Vertex 7 (Color 1).
Vertex 6 (Color 0) is connected to Vertex 3 (Color 2), Vertex 10 (Color 1) and 13 (Color 2), but also to Vertex 8 (Color 2).
============================
The coloring is incorrect. Vertex 1 (Color 2) and Vertex 3 (Color 3) are connected but have different colors. Vertex 3 (Color 3) is connected to Vertex 6 (Color 3).
============================
Vertex 10, colored 4, is connected to vertex 11, also colored 1. However, it is also colored 4, which is greater than the optimal coloring of 4. So, this coloring is non-optimal.
