# Supplementary material for: GPT-4 Doesn't Know It's Wrong: An Analysis of Iterative Prompting for Reasoning Problems
Source: arXiv:2310.12397 source file (2023-10-19)
Supplement: Supplementary file 5 [file dimacs_example.tex]

e 0 7
e 0 8
e 0 9
e 0 11
e 1 13
e 2 9
e 3 8
e 3 11
e 3 12
e 4 12
e 5 11
e 6 9
e 7 10
e 7 13
e 9 11
e 10 13
e 11 13
c OPTIMAL CHROMATIC NUMBER === 3
