# Supplementary material for: GPT-4 Doesn't Know It's Wrong: An Analysis of Iterative Prompting for Reasoning Problems
Source: arXiv:2310.12397 source file (2023-10-19)
Supplement: Supplementary file 10 [file passfail_example_backprompt.tex]

This is not correct. Using the previously provided graph, please provide a correct coloring. Please provide each vertex's color. Do not skip any vertices. Each color must be provided on a new line in the response and should be formatted as "{VERTEX NUMBER}: {VERTEX COLOR ASSIGNMENT}". Please do not provide anything else in your response.
